# Supplementary material for: Cross-Matched Interval Prevalence of High Dimensional Point Clouds
Source: arXiv:2411.09797 source file (2024-11-14)
Supplement: Supplementary file 1 [file X_suppl.tex]

\clearpage
\setcounter{page}{1}
\maketitlesupplementary

\subsection{Clustering Algorithm}

\subsection{Additional Experiments}
